# Supplementary material for: Mirror Descent Policy Optimization
Source: arXiv:2005.09814 source file (2021-06-07)
Supplement: Supplementary file 1 [file Appendix.tex]

\clearpage
%%%%%%%%%%%%%%%%%%%%%%%%%%%%%%%%%%%%%%%%%%%%%%%%%%%%%%%%%%%%
